# Supplementary material for: Eyes Can't Always Tell: Fusing Eye Tracking and User Priors for User Modeling under AI Advice Conditions
Source: arXiv:2604.01741 source file (2026-06-25)
Supplement: Supplementary file 1 [file appendix.tex]

\clearpage
\onecolumn

% ===================================================

% \begin{appendices}
% \renewcommand{\thesection}{Appendix A}

\setcounter{table}{0} % Reset table counter
\setcounter{figure}{0} % Reset table counter

\section*{Supplement A: Examples of Stimuli}
\label{sec:appendix_stimuli_examples}

% \clearpage
% \onecolumn

\begin{table*}[!h]
\centering
\footnotesize

\begin{tabularx}{\textwidth}{>{\raggedright\arraybackslash}p{0.22\textwidth} >
{\raggedright\arraybackslash}X} 
\hline
\multicolumn{1}{l}{\textbf{Component}} & \multicolumn{1}{l}{\textbf{Content}} \\
\hline

\textbf{Factual Verification Question} & 
Is Miami a city on the American West Coast?
\\ \hline

% \textbf{AI's Answer} & 
% No, Miami is not a city on the American West Coast. 
% It's located in Florida, which is part of the southeastern region of the United States and lies along the East Coast.
% \\ \cline{1-2}

\textbf{AI's Advice\newline(Correct)} &  
% First, let’s identify where Miami is located. 
Miami is a city in the state of Florida, and it sits in the southeastern part of the United States along the Atlantic Ocean.\newline
% Now, let’s consider what is meant by the American West Coast. This term refers to the coastal states bordering the Pacific Ocean—California, Oregon, Washington, Alaska, and sometimes Hawaii. 
Since Florida is located on the East Coast, it is not part of the West Coast. Therefore, Miami is not a city on the American West Coast.
\\ \cline{1-2}

\textbf{AI's Advice\newline(Incorrect)} &  
Miami is located in the state of California, which is one of the primary West Coast states. (Here is the factual incorrectness in this step)\newline
American West Coast refers to the coastal states bordering the Pacific Ocean, California, Oregon, Washington, Alaska, and sometimes Hawaii. 
% Despite that, when we review the actual location of Miami, it's evident that it’s not on the Pacific Ocean but on the Atlantic, which confirms it’s not a city on the West Coast.\newline
So Miami is on the American West Coast.
\\ \hline
\end{tabularx}
\caption{An example factual verification question and the AI advice shown to participants: the advice is either correct or incorrect, depending on the condition.}
\vspace{-6.6mm}
\end{table*}

% ===================================================

% \end{appendices}
